# Supplementary material for: A Convergence Theory Towards Practical Over-parameterized Deep Neural Networks
Source: arXiv:2101.04243 source file (2021-02-08)
Supplement: Supplementary file 3 [file appendix-20200923.tex]

\newpage
\begin{center} \begin{huge}{Appendix} \end{huge} \end{center}
\label{appendix}
\section{Auxiliary Lemmas}
\begin{lemma} \label{lemma:1}
Define
\[
    \I_k^i = \left\{s \in [m]: [\Psi_k x_i]_s > 0 \right \}, \quad \I_k^j = \left\{s \in [m]: [\Psi_k x_j]_s > 0 \right \}
\]
where $\Psi_k \in \R^{m\times m}$ is a Gaussian random matrix. Suppose $\nm{x_i^{\top}x_j} \leq \delta$, where $\delta \leq 1/3$. Then, with a probability $1 - \exp(-\Omega(m))$, we have
\[
    \left|\I_k^i \cap \I_k^j \right| \leq \frac{m}{3}
\]
\end{lemma}
\begin{proof}
Define $[z]_+$ that outputs $1$ when $z > 0$, and zero otherwise. We have
\begin{eqnarray*}
    \left|\I_k^j \cap \I_k^i\right| & = & \langle\left[\Psi_kx_j\right]_+, \left[\Psi_kx_i\right]_+ \rangle \\
    & \leq & \langle\left[\Psi_kx_j\right]_+, \left[\Psi_k\left(x_i - P_{x_j}(x_i)\right)\right]_+ \rangle + \left|\left[\Psi_kx_i\right]_+ - \left[\Psi_k\left(x_i - P_{x_j}(x_i)\right)\right]_+\right|
\end{eqnarray*}
Since $\Psi_k(x_i - P_{x_j}(x_i))$ and $\Psi_k x_j$ are statistically independent, hence, with a probability $1 - \exp(-\epsilon m/2)$,
\[
\langle \left[\Psi x_j\right]_+, \left[\Psi_k(x_i - P_{x_j}(x_i)\right]_+\rangle \leq \frac{(1+\epsilon)m}{4}
\]
and therefore,
\begin{eqnarray*}
\lefteqn{\left|\I_k^j \cap \I_k^i\right|} \\
& \leq & \frac{(1+\epsilon)m}{4} + \left|\left[\Psi_kx_i\right]_+ - \left[\Psi_k\left(x_i - P_{x_j}(x_i)\right)\right]_+\right| \\
& \leq & \frac{(1+\epsilon)m}{4} + \underbrace{\sum_{\ell=1}^m I\left(\left|\left[\Psi_kP_{x_j}(x_i)\right]_{\ell}\right| > \left|\left[\Psi_k\left(x_i - P_{x_j}(x_i)\right)\right]_{\ell}\right|\right)}_{:= Z}
\end{eqnarray*}
We proceed to bound $Z$. First, each element of $\Psi_k P_{x_j}(x_i)$ follows a Gaussian distribution $\N(0, \sigma_1^2)$, where $\sigma_1^2 = 2|\Psi_k P_{x_j}(x_i)|^2/m$. Similarly, each element $\Psi_k (x_i - P_{x_j}(x_i))$ follows a distribution $\N(0, \sigma_2^2)$, where $\sigma_2^2 = 2|\Psi_k(x_i - P_{x_j}(x_i))|^2/m$. Using the concentration inequality of $\chi^2_m$ distribution, we have, with a probability $1 - 2\exp(-\epsilon m/4)$,
\[
    \sigma_1^2 \leq \frac{2(1+\epsilon)}{m}\left|P_{x_j}(x_i)\right|^2\leq\frac{2(1+\epsilon)\delta^2}{m}, \quad \sigma_2^2 \geq \frac{2(1-\epsilon)}{m}\left|\left(x_i - P_{x_j}(x_i)\right)\right|^2 \geq \frac{2(1-\epsilon)(1 - \delta^2)}{m}
\]
Using the properties of Gaussian distribution, we have
\begin{eqnarray*}
    \lefteqn{\Pr\left(\left|\left[\Psi_k\left(x_i - P_{x_j}(x_i)\right)\right]_{\ell}\right|^2 \geq \frac{2\delta}{m}\sqrt{\frac{(1 - \epsilon)(1-\delta^2)}{1+\epsilon}}\right)} \\
    & \geq & 1 - \left(\frac{(1+\epsilon)\delta^2}{(1-\epsilon)1 - \delta^2}\right)^{1/4} \exp\left(-\frac{1 - \left[(1+\epsilon)\delta^2/[(1 - \epsilon)(1-\delta^2)]\right]^{1/4}}{2}\right) \geq 1 - 2\delta^{1/4}
\end{eqnarray*}
\begin{eqnarray*}
    \lefteqn{\Pr\left(\left|\left[\Psi_k P_{x_j}(x_i)\right]_{\ell}\right|^2 \geq \frac{2\delta}{m}\sqrt{\frac{(1 - \epsilon)(1 - \delta^2)}{1+\epsilon}}{m}\right)} \\
     & \leq & \left(\frac{(1-\epsilon)(1 - \delta^2)}{(1 + \epsilon)\delta^2}\right)^{1/4} \exp\left(- \frac{\left[(1 - \epsilon)(1 - \delta^2)/(1+\epsilon)\delta^2\right]^{1/4}}{2}\right) \leq \exp\left(-\frac{1}{2\delta}\right)
\end{eqnarray*}
As a result, we have
\[
\Pr\left(\left|\left[\Psi_k\left(x_i - P_{x_j}(x_i)\right)\right]_{\ell}\right| < \left|\left[\Psi_k P_{x_j}(x_i)\right]_{\ell}\right|\right) \leq 3\delta^{1/4}\exp\left(-\frac{1}{2\delta}\right)
\]
Using the standard concentration inequality, we have, with a probability $1 - \exp(-m/2)$,
\[
    Z \leq \left(2\delta^{1/4}\exp\left(-\frac{1}{2\delta}\right) + \frac{1}{3.5}\right)m + 2m\sqrt{\delta^{1/4}\exp\left(-\frac{1}{2\delta}\right)} \leq \frac{m}{7}
\]
and therefore, with a probability $1 - \exp(-\Omega(m))$, we have
\[
\left|\I_k^j \cap \I_k^i\right| \leq \frac{m}{3}
\]
\end{proof}
\asaf{why? $\frac{1}{4}+\frac{1}{7}>\frac{1}{3}$}
\asaf{if two examples has some corr, wouldn't it quickly decrease to zero during forward?}
% \begin{lemma}\label{lemma:z-ka-kb}
% Define 
% \[
% Z_{k_a, k_b} = D_{k_a}^iW_{1,k_a}\ldots W_{1,k_b+1}D_{k_b}^i
% \]
% With a probability at least $1 - 2L^2\sqrt{m}\exp\left(-\epsilon m/[4L] + 6\sqrt{m}\right)$, for any $1 \leq k_b \leq k_a \leq L$ and any $\epsilon \in (0, 1/5)$, we have
% \[
%     \nm{Z_{k_a,k_b}} _2\leq \sqrt{3}m^{1/4}e^{\epsilon/2}
% \]
% and
% \[
%     \min\limits_{\|v\| \geq 1}\|Z_{k_a,k_b}v\| \geq e^{-\epsilon}m^{1/4}
% \]
% \asaf{Doesn't the lower bound contradicts the new log-bound?}
% \end{lemma}
% %\end{lemma}
% \begin{proof}
% To bound $\|Z_{k_a, k_b}\|_2$, we will bound $\max\limits_{\nm{v} \leq 1} \nm{Z_{k_a, k_b}v}$. To this end, we divide $v$ into $\sqrt{m}$ components of equal size, denoted by $v_1, \ldots, v_{\sqrt{m}}$. We furthermore introduce $\tilde{v}_k \in \R^m$ to include the $k$th component $v_k$ of $v$ with everything else padded with zeros. As a result,
% \begin{eqnarray*}
%     \max\limits_{\nm{v} \leq 1} \nm{Z_{k_a,k_b}v} &\leq& \max\limits_{\sum_{j=1}^{\sqrt{m}} \nm{v_j}^2 \leq 1} \sum_{j=1}^{\sqrt{m}} \nm{Z_{k_a,k_b}\tilde{v}_j} \\ 
%     &\leq& \max\limits_{\sum_{j=1}^{\sqrt{m}}\nm{v_j}^2 \leq 1} \sum_{j=1}^{\sqrt{m}}\nm{v_j}\max_{v_j \in \R^{\sqrt{m}}} \frac{\nm{Z_{k_a,k_b} \tilde{v}_j}}{\nm{v_j}} = m^{1/4}\max_{j \in [\sqrt{m}], v_j \in \R^{\sqrt{m}}} \frac{\nm{Z_{k_a,k_b} \tilde{v}_j}}{\nm{v_j}}
% \end{eqnarray*}
% We fix $j$ and consider a fixed $\tilde{v}_j \in \R^{\sqrt{m}}$. We will prove the following high probability bound by induction
% \[
% \nm{Z_{k_a, k_b} \tilde{v}_j}^2 \in \left(\left(1 - \frac{\epsilon}{L}\right)^{k_a - k_b}\nm{D_{k_b}^i\tilde{v}_j}^2, \left(1 + \frac{\epsilon}{L}\right)^{k_b-k_a}\nm{D_{k_b}^i\tilde{v}_j}^2\right).
% \]
% where $\epsilon \in (0, 1/2)$ is a introduced parameter related to the failure probability. For $k_a = k_b +1$, we have
% \[
%     \nm{Z_{k_a, k_b}\tilde{v}_j}^2 = \nm{D^i_{k_b+1} W_{1,k_b+1} D^i_{k_b} \tilde{v}_j}^2
% \]
% It is easy to show that $\nm{Z_{k_a, k_b}\tilde{v}_j}^2$ follows the distribution of $\frac{2}{m}\nm{D^i_{k_b}\tilde{v}_j}^2\chi^2_{m/2}$. Using the concentration of $\chi^2$ distribution, we have
% \[
%     \Pr\left(\nm{Z_{k_a,k_b}\tilde{v}_j}^2 \geq \left(1 + \frac{\epsilon}{L}\right)\nm{D^i_{k_b}\tilde{v}_j}^2\right) \leq \exp\left(-\frac{\epsilon m}{4L}\right)
% \]
% and
% \[
%     \Pr\left(\nm{Z_{k_a,k_b}\tilde{v}_j}^2 \leq \left(1 - \frac{\epsilon}{L}\right)\nm{D^i_{k_b}\tilde{v}_j}^2\right) \leq \exp\left(-\frac{\epsilon m}{4L}\right)
% \]
% \asaf{The factor of $2$ is possibly not handled well.}
% Hence, with a probability $1 - 2 \exp(-\epsilon m/[4L])$, we have
% \[
%     \nm{Z_{k_a, k_b}\tilde{v}_j}^2 \in\left[\left(1- \frac{\epsilon}{L}\right)\nm{D_{k_b}^i \tilde{v}_j}^2, \left(1 + \frac{\epsilon}{L}\right)\nm{D_{k_b}^i \tilde{v}_j}^2\right]
% \]
% The inductive step will follow the same argument. As a result, for a fixed $\tilde{v}_j$, for any $k_a$ and $k_b$, with a probability $1 - 2L^2\exp(-\epsilon m/[4L])$, we have
% \[
%   \nm{Z_{k_a, k_b} \tilde{v}_j}^2 \in \left[\left(1 - \frac{\epsilon}{L}\right)^L\nm{D^i_{k_b}\tilde{v}_j}^2, \left(1 + \frac{\epsilon}{L}\right)^L\nm{D_{k_b}^i \tilde{v}_j}^2\right]
% \]
% Since $\epsilon < 1/5$, the above bound can be simplified as
% \[
%     \nm{Z_{k_a, k_b} \tilde{v}_j}^2 \in \left[e^{-2\epsilon}\nm{D^i_{k_b}\tilde{v}_j}^2, e^{\epsilon}\nm{D_{k_b}^i \tilde{v}_j}^2\right]
% \]

% To bound $\nm{Z_{k_a, k_b}\tilde{v}_j}^2$ for any $\tilde{v}_j$, we introduce $\N \subset \mathcal{S}^{\sqrt{m} - 1}$ as an appropriate $\varepsilon$-net of $\mathcal{S}^{\sqrt{m} - 1}$. Using the well known property of appropriate $\varepsilon$-net, we have
% \[
%     \max\limits_{v_j \in \N} \nm{Z_{k_a, k_b}\tilde{v}_j}^2 \leq \max\limits_{v_j \in \R^{\sqrt{m} - 1}} \frac{\nm{Z_{k_a, k_b}\tilde{v}_j}^2}{\nm{v_j}^2} \leq \frac{1}{1 - 2\varepsilon}\max\limits_{v_j \in \N} \nm{Z_{k_a, k_b}\tilde{v}_j}^2
% \]
% Since $|\N| \leq (1 + 2/\varepsilon)^{\sqrt{m}} \leq \exp(2\sqrt{m}/\varepsilon)$, by taking the union bound, we have, with probability at least $ 1- 2L^2\exp(-\epsilon m/[4L] + 2\sqrt{m}/\varepsilon)$,
% \[
% \max\limits_{v_j \in \R^{\sqrt{m} - 1}} \frac{\nm{Z_{k_a, k_b}\tilde{v}_j}^2}{\nm{v_j}^2} \in \left[e^{-2\epsilon}\frac{\nm{D^i_{k_b}\tilde{v}_j}^2}{\nm{v_j}^2}, \frac{e^{\epsilon}}{1 - 2\varepsilon}\frac{\nm{D^i_{k_b}\tilde{v}_j}^2}{\nm{v_j}^2} \right]
% \]
% By choosing $\varepsilon = 1/3$ and $\epsilon < 1/2$, we have, with a probability at least $ 1- 2L^2\exp(-\epsilon m/[4L] + 6\sqrt{m})$
% \[
% \max\limits_{v_j \in \R^{\sqrt{m} - 1}} \frac{\nm{Z_{k_a, k_b}\tilde{v}_j}^2}{\nm{v_j}^2} \in \left[e^{-2\epsilon}\frac{\nm{D^i_{k_b}\tilde{v}_j}^2}{\nm{v_j}^2}, 3e^{\epsilon}\frac{\nm{D^i_{k_b}\tilde{v}_j}^2}{\nm{v_j}^2} \right].
% \]
% and therefore, with a probability $ 1- L^2\sqrt{m}\exp(-\epsilon m/[4L] + 6\sqrt{m})$, for any $1\leq k_b < k_a \leq L$, we have
% \[
% \nm{Z_{k_a, k_b}}_2 \leq \sqrt{3}m^{1/4}e^{\epsilon/2}
% \]
% \end{proof}

\begin{lemma}\label{lemma:z-ka-kb}
Define 
\[
Z_{k_a, k_b} = D_{k_a}^iW_{1,k_a}\ldots W_{1,k_b+1}D_{k_b}^i
\]
With a probability at least $ 1- 18L^3\varepsilon^{-2}\exp(-\epsilon m/[36L])$, for any $1 \leq k_b \leq k_a \leq L$ and any $\epsilon \in (0, 1/5)$, we have
\[
    \nm{Z_{k_a, k_b}}_2 \leq \sqrt{15L}\varepsilon^{-1} e^{\epsilon/2}
\]
\end{lemma}
\begin{proof}
To bound $\|Z_{k_a, k_b}\|_2$, we will bound $\max\limits_{\nm{v} \leq 1} \nm{Z_{k_a, k_b}v}$. To this end, we divide $v$ into 
% $r=\left\lceil{\max\braces{\log^2{m},4L/\brackets{\varepsilon^2}}}\right \rceil$ 
$r=\left\lceil{9L/\brackets{\varepsilon^2}}\right \rceil$
components of equal size (last is possibly smaller), denoted by $v_1, \ldots, v_{r}$. We furthermore introduce $\tilde{v}_k \in \R^m$ to include the $k$th component $v_k$ of $v$ with everything else padded with zeros. As a result,
\begin{eqnarray*}
    \max\limits_{\nm{v} \leq 1} \nm{Z_{k_a,k_b}v} &\leq& \max\limits_{\sum_{j=1}^{r} \nm{v_j}^2 \leq 1} \sum_{j=1}^{r} \nm{Z_{k_a,k_b}\tilde{v}_j} \\ 
    &\leq & \max\limits_{\sum_{j=1}^{r}\nm{v_j}^2 \leq 1} \sum_{j=1}^{r}\nm{v_j}\max_{v_j \in \R^{m/r}} \frac{\nm{Z_{k_a,k_b} \tilde{v}_j}}{\nm{v_j}} \\
    & = & \sqrt{r}\max_{j \in [r], v_j \in \R^{m/r}} \frac{\nm{Z_{k_a,k_b} \tilde{v}_j}}{\nm{v_j}}
\end{eqnarray*}
We fix $j$ and consider a fixed $\tilde{v}_j \in \R^{m/r}$. We will prove the following high probability bound by induction
\[
\nm{Z_{k_a, k_b} \tilde{v}_j}^2 \in \left(\left(1 - \frac{\epsilon}{L}\right)^{k_a - k_b}\nm{D_{k_b}^i\tilde{v}_j}^2, \left(1 + \frac{\epsilon}{L}\right)^{k_b-k_a}\nm{D_{k_b}^i\tilde{v}_j}^2\right).
\]
where $\epsilon \in (0, 1/2)$ is a introduced parameter related to the failure probability. For $k_a = k_b +1$, we have
\[
    \nm{Z_{k_a, k_b}\tilde{v}_j}^2 = \nm{D^i_{k_b+1} W_{1,k_b+1} D^i_{k_b} \tilde{v}_j}^2
\]
It is easy to show that $\nm{Z_{k_a, k_b}\tilde{v}_j}^2$ follows the distribution of $\frac{2}{m}\nm{D^i_{k_b}\tilde{v}_j}^2\chi^2_{m/2}$. Using the concentration of $\chi^2$ distribution, we have
\[
    \Pr\left(\nm{Z_{k_a,k_b}\tilde{v}_j}^2 \geq \left(1 + \frac{\epsilon}{L}\right)\nm{D^i_{k_b}\tilde{v}_j}^2\right) \leq \exp\left(-\frac{\epsilon m}{4L}\right)
\]
and
\[
    \Pr\left(\nm{Z_{k_a,k_b}\tilde{v}_j}^2 \leq \left(1 - \frac{\epsilon}{L}\right)\nm{D^i_{k_b}\tilde{v}_j}^2\right) \leq \exp\left(-\frac{\epsilon m}{4L}\right)
\]
%\asaf{The factor of $2$ is possibly not handled well.}
Hence, with a probability $1 - 2 \exp(-\epsilon m/[4L])$, we have
\[
    \nm{Z_{k_a, k_b}\tilde{v}_j}^2 \in\left[\left(1- \frac{\epsilon}{L}\right)\nm{D_{k_b}^i \tilde{v}_j}^2, \left(1 + \frac{\epsilon}{L}\right)\nm{D_{k_b}^i \tilde{v}_j}^2\right]
\]
The inductive step will follow the same argument. As a result, for a fixed $\tilde{v}_j$, for any $k_a$ and $k_b$, with a probability $1 - 2L^2\exp(-\epsilon m/[4L])$, we have
\[
   \nm{Z_{k_a, k_b} \tilde{v}_j}^2 \in \left[\left(1 - \frac{\epsilon}{L}\right)^L\nm{D^i_{k_b}\tilde{v}_j}^2, \left(1 + \frac{\epsilon}{L}\right)^L\nm{D_{k_b}^i \tilde{v}_j}^2\right]
\]
Since $\epsilon < 1/5$, the above bound can be simplified as
\[
    \nm{Z_{k_a, k_b} \tilde{v}_j}^2 \in \left[e^{-2\epsilon}\nm{D^i_{k_b}\tilde{v}_j}^2, e^{\epsilon}\nm{D_{k_b}^i \tilde{v}_j}^2\right]
\]

To bound $\nm{Z_{k_a, k_b}\tilde{v}_j}^2$ for any $\tilde{v}_j$, we introduce $\N \subset \mathcal{S}^{m/r - 1}$ as an appropriate $\varepsilon$-net of $\mathcal{S}^{m/r - 1}$. Using the well known property of appropriate $\varepsilon$-net, we have
\[
    \max\limits_{v_j \in \N} \nm{Z_{k_a, k_b}\tilde{v}_j}^2 \leq \max\limits_{v_j \in \R^{m/log^2m - 1}} \frac{\nm{Z_{k_a, k_b}\tilde{v}_j}^2}{\nm{v_j}^2} \leq \frac{1}{1 - 2\varepsilon}\max\limits_{v_j \in \N} \nm{Z_{k_a, k_b}\tilde{v}_j}^2
\]
Since $|\N| \leq (1 + 2/\varepsilon)^{m/r} \leq \exp(2m/[\varepsilon r])$, by taking the union bound, we have, with probability at least $ 1- 2L^2\exp(-\epsilon m/[36L])$,
\[
\max\limits_{v_j \in \R^{\sqrt{m} - 1}} \frac{\nm{Z_{k_a, k_b}\tilde{v}_j}^2}{\nm{v_j}^2} \in \left[e^{-2\epsilon}\frac{\nm{D^i_{k_b}\tilde{v}_j}^2}{\nm{v_j}^2}, \frac{e^{\epsilon}}{1 - 2\varepsilon}\frac{\nm{D^i_{k_b}\tilde{v}_j}^2}{\nm{v_j}^2} \right]
\]
Since $\epsilon < 1/5$, we have, with a probability at least $ 1- 2L^2\exp(-\epsilon m/[36L])$
\[
\max\limits_{v_j \in \R^{\sqrt{m} - 1}} \frac{\nm{Z_{k_a, k_b}\tilde{v}_j}^2}{\nm{v_j}^2} \in \left[e^{-2\epsilon}\frac{\nm{D^i_{k_b}\tilde{v}_j}^2}{\nm{v_j}^2}, \frac{5}{3}e^{\epsilon}\frac{\nm{D^i_{k_b}\tilde{v}_j}^2}{\nm{v_j}^2} \right].
\]
and therefore, with a probability $ 1- 18L^3\varepsilon^{-2}\exp(-\epsilon m/[36L])$, for any $1\leq k_b < k_a \leq L$, we have
% \[
% \nm{Z_{k_a, k_b}}_2 \leq \sqrt{3}\log m e^{\epsilon/2}
% \]
% \[
% \nm{Z_{k_a, k_b}}_2 \leq \sqrt{3}\frac{4\sqrt{L}}{\varepsilon} e^{\epsilon/2}
% \]
\[
\nm{Z_{k_a, k_b}}_2 \leq \sqrt{15L}\varepsilon^{-1} e^{\epsilon/2}
\]
\end{proof}

%-------Rewrite lemma 4, only upper bound.
\begin{lemma}\label{lemma:z-ka-kb-2}
(a) For any $1 \leq k_b \leq k_a \leq L$, we have, 
\[
    \nm{Z_{k_a,k_b}} _2\leq 19\sqrt{L} \quad \textrm{with a probability (w.p) of at least}~  1- 81L^3\exp(- m/[108L])
\]
(b)  with a probability at least $1- 2L^2\exp(-\epsilon m/[4L] +3d_x)$,
\[ \min\limits_{u \in \R^d}\frac{\nm{Z_{k_a, k_b} C u}}{\nm{u}} \geq \sqrt{\frac{m}{3d_x}}e^{-\epsilon} \quad
\textrm{and} \quad
\max\limits_{u \in \R^d}\frac{\nm{Z_{k_a, k_b} C u}}{\nm{u}} \geq \sqrt{\frac{3m}{d_x}}e^{\epsilon/2} \textrm{w.p}~ 1- 2L^2\exp(-\epsilon m/[4L] +3d_x)
\]
\end{lemma}
\begin{proof}
(a) To bound $\|Z_{k_a, k_b}\|_2$, we will bound $\max\limits_{\nm{v} \leq 1} \nm{Z_{k_a, k_b}v}$. To this end, we divide $v$ into 
% $r=\left\lceil{\max\braces{\log^2{m},4L/\brackets{\varepsilon^2}}}\right \rceil$ 
$r=\left\lceil{9L/\brackets{\varepsilon^2}}\right \rceil$
components of equal size (last is possibly smaller), denoted by $v_1, \ldots, v_{r}$. We furthermore introduce $\tilde{v}_k \in \R^m$ to include the $k$th component $v_k$ of $v$ with everything else padded with zeros. As a result,
\begin{eqnarray*}
    \max\limits_{\nm{v} \leq 1} \nm{Z_{k_a,k_b}v} &\leq& \max\limits_{\sum_{j=1}^{r} \nm{v_j}^2 \leq 1} \sum_{j=1}^{r} \nm{Z_{k_a,k_b}\tilde{v}_j} \\ 
    &\leq & \max\limits_{\sum_{j=1}^{r}\nm{v_j}^2 \leq 1} \sum_{j=1}^{r}\nm{v_j}\max_{v_j \in \R^{m/r}} \frac{\nm{Z_{k_a,k_b} \tilde{v}_j}}{\nm{v_j}} \\
    & = & \sqrt{r}\max_{j \in [r], v_j \in \R^{m/r}} \frac{\nm{Z_{k_a,k_b} \tilde{v}_j}}{\nm{v_j}}
\end{eqnarray*}
We fix $j$ and consider a fixed $\tilde{v}_j \in \R^{m/r}$. We prove the following high probability bound by induction for $\varepsilon>0$, related to the failure probability,
\[
\nm{Z_{k_a, k_b} \tilde{v}_j}^2 \leq \left(1 + \frac{\epsilon}{L}\right)^{k_b-k_a}\nm{D_{k_b}^i\tilde{v}_j}^2
\]
% where $\epsilon \in (0, 1/2)$ is a introduced parameter related to the failure probability. 
For $k_a = k_b +1$, we have
\[
    \nm{Z_{k_a, k_b}\tilde{v}_j}^2 = \nm{D^i_{k_b+1} W_{1,k_b+1} D^i_{k_b} \tilde{v}_j}^2
\]
It is easy to show that $\nm{Z_{k_a, k_b}\tilde{v}_j}^2$ follows the distribution of $\frac{2}{m}\nm{D^i_{k_b}\tilde{v}_j}^2\chi^2_{m/2}$. Using the concentration of $\chi^2$ distribution, we have
\[
    \Pr\left(\nm{Z_{k_a,k_b}\tilde{v}_j}^2 \geq \left(1 + \frac{\epsilon}{L}\right)\nm{D^i_{k_b}\tilde{v}_j}^2\right) \leq \exp\left(-\frac{\epsilon m}{4L}\right)
\]
% and
% \[
%     \Pr\left(\nm{Z_{k_a,k_b}\tilde{v}_j}^2 \leq \left(1 - \frac{\epsilon}{L}\right)\nm{D^i_{k_b}\tilde{v}_j}^2\right) \leq \exp\left(-\frac{\epsilon m}{4L}\right)
% \]
% %\asaf{The factor of $2$ is possibly not handled well.}
% Hence, with a probability $1 - 2 \exp(-\epsilon m/[4L])$, we have
% \[
%     \nm{Z_{k_a, k_b}\tilde{v}_j}^2 \in\left[\left(1- \frac{\epsilon}{L}\right)\nm{D_{k_b}^i \tilde{v}_j}^2, \left(1 + \frac{\epsilon}{L}\right)\nm{D_{k_b}^i \tilde{v}_j}^2\right]
% \]
The inductive step will follow the same argument. As a result, for a fixed $\tilde{v}_j$, for any $k_a$ and $k_b$, with a probability $1 - L^2\exp(-\epsilon m/[4L])$, we have
\[
   \nm{Z_{k_a, k_b} \tilde{v}_j}^2 \leq \left(1 + \frac{\epsilon}{L}\right)^L\nm{D_{k_b}^i \tilde{v}_j}^2 \leq e^{\epsilon}\nm{D_{k_b}^i \tilde{v}_j}^2 
\]
% Since $\epsilon < 1/5$, the above bound can be simplified as
% \[
%     \nm{Z_{k_a, k_b} \tilde{v}_j}^2 \in \left[e^{-2\epsilon}\nm{D^i_{k_b}\tilde{v}_j}^2, e^{\epsilon}\nm{D_{k_b}^i \tilde{v}_j}^2\right]
% \]

To bound $\nm{Z_{k_a, k_b}\tilde{v}_j}^2$ for any $\tilde{v}_j$, we introduce $\N \subset \mathcal{S}^{m/r - 1}$ as an appropriate $\varepsilon$-net of $\mathcal{S}^{m/r - 1}$. Using the well known property of appropriate $\varepsilon$-net, we have
\[
    \max\limits_{v_j \in \N} \nm{Z_{k_a, k_b}\tilde{v}_j}^2 \leq \max\limits_{v_j \in \R^{m/log^2m - 1}} \frac{\nm{Z_{k_a, k_b}\tilde{v}_j}^2}{\nm{v_j}^2} \leq \frac{1}{1 - 2\varepsilon}\max\limits_{v_j \in \N} \nm{Z_{k_a, k_b}\tilde{v}_j}^2
\]
Since $|\N| \leq (1 + 2/\varepsilon)^{m/r} \leq \exp(2m/[\varepsilon r])$, by taking the union bound, we have, with probability at least $ 1- L^2\exp(-\epsilon m/[36L])$,
\[
\max\limits_{v_j \in \R^{\sqrt{m} - 1}} \frac{\nm{Z_{k_a, k_b}\tilde{v}_j}^2}{\nm{v_j}^2} \leq \frac{e^{\epsilon}}{1 - 2\varepsilon}\frac{\nm{D^i_{k_b}\tilde{v}_j}^2}{\nm{v_j}^2} 
\]
% Since $\epsilon < 1/5$, we have, with a probability at least $ 1- 2L^2\exp(-\epsilon m/[36L])$
% \[
% \max\limits_{v_j \in \R^{\sqrt{m} - 1}} \frac{\nm{Z_{k_a, k_b}\tilde{v}_j}^2}{\nm{v_j}^2} \in \left[e^{-2\epsilon}\frac{\nm{D^i_{k_b}\tilde{v}_j}^2}{\nm{v_j}^2}, \frac{5}{3}e^{\epsilon}\frac{\nm{D^i_{k_b}\tilde{v}_j}^2}{\nm{v_j}^2} \right].
% \]
For $\varepsilon=1/3$, with a probability $ 1- 81L^3\exp(- m/[108L])$, for any $1\leq k_b < k_a \leq L$, we have
% \[
% \nm{Z_{k_a, k_b}}_2 \leq \sqrt{3}\log m e^{\epsilon/2}
% \]
% \[
% \nm{Z_{k_a, k_b}}_2 \leq \sqrt{3}\frac{4\sqrt{L}}{\varepsilon} e^{\epsilon/2}
% \]
\[
\nm{Z_{k_a, k_b}}_2 \leq \sqrt{9L}\varepsilon^{-1}(1-2\varepsilon)^{-0.5} e^{\epsilon/2} \leq 19\sqrt{L}
\]
(c) Same as (a) and (b), only with $r=d_x$
\end{proof}
%---------

\begin{lemma} \label{lemma:z-ka-kb-t}
Under the following assumption,
\[
    \sqrt{3}e^{\epsilon/2}m^{1/4}L\tau \leq \frac{1}{9}
\]
%Then, for any
with some $\epsilon \in (0, 1/5)$. Then, for any $1 \leq k_b < k_b \leq L$, with a probability larger than $1 - L^2\sqrt{m}\exp\left(-\epsilon m/[4L] + 6\sqrt{m}\right)$ we have
\[
    \|Z_{k_a, k_b}^t\|_2 \leq 5e^{\epsilon/2}m^{1/4}
\]
\end{lemma}
\begin{proof}
Define $Z_{k,k'} = D_k^iW_{1,k}\ldots W_{1,k'+1}D_{k'}^i$
and $\delta W_{t,k} = W_{t,k} - W_{1,t}$. Expand $Z^t_{k_a, k_b}$ as
\begin{eqnarray*}
Z_{k_a,k_b}^t = Z_{k_a, k_b} + \sum_{s=1}^{k_b - k_a} \sum_{k_1 > k_2 >\ldots > k_s}Z_{k_a, k_1+1}\prod_{\ell=1}^s\delta W_{t,k_{\ell}}Z_{k_{\ell}+1, k_{\ell+1}}
\end{eqnarray*}
According to Lemma~\ref{lemma:z-ka-kb}, for any $\epsilon \in (0, 1/5)$, with a probability $1 - \sqrt{m}\exp\left(-\epsilon m/[4L] + 6\sqrt{m}\right)$, we have $\|Z_{k,k'}\| \leq \sqrt{3}m^{1/4}e^{\epsilon/2}$. We thus have, with a probability $1 - L^2\sqrt{m}\exp\left(-\epsilon m/[4L] + 6\sqrt{m}\right)$, \begin{eqnarray*}
\|Z^t_{k_a, k_b}\|_2 \leq \sqrt{3}e^{\epsilon/2}m^{1/4}\left(1 + \sum_{s=1}^L \left[\sqrt{3}e^{\epsilon/2}m^{1/4}L\tau\right]^s\right) \leq \sqrt{3}e^{\epsilon/2}m^{1/4}\left(1 + \frac{1}{1 - \sqrt{3}e^{\epsilon/2}m^{1/4}L\tau}\right)
\end{eqnarray*}
Since
\[
\sqrt{3}e^{\epsilon/2}m^{1/4}L\tau \leq \frac{1}{9}
\]
\asaf{I think the it should be $c(1+\frac{q}{1-q})$ so $\frac{9\sqrt{3}}{8}$ and not $\frac{17\sqrt{3}}{8}$, and below $5\rightarrow 2$}
we have
\[
    \|Z^t_{k_a, k_b}\|_2 \leq 5e^{\epsilon/2}m^{1/4}
\]
\end{proof}
% \asaf{Only upper bounding Z for now:}
% \begin{lemma} \label{lemma:z-ka-kb-t_log_bound}
% Define for every $i\in[n]$, and $1 \leq k_b \leq k_a \leq L$,
% \[
% Z^i_{k_a, k_b} = D_{k_a}^iW_{1,k_a}\ldots W_{1,k_b+1}D_{k_b}^i
% \]
%  Then for every $\varepsilon>0$ with a probability of at least %$1-mL^2\paren{2\exp\left(-\frac{m\varepsilon^2}{8L^2}\right) +\brackets{e^{2\varepsilon-1}\log m}^{-\log m}}$,
% TBD,
% \begin{eqnarray} 
%     \nm{Z^i_{k_a, k_b} } _2\leq C\log m
% \end{eqnarray} 
% \end{lemma}
% \begin{proof}
% We start by stating a lemma for bounding the spectral norm of a sum of independent random matrices,
% \begin{lemma}[Matrix Chernoff bound, \cite{tropp2012user} Remark $5.3$] \label{lemma:tropp_2010}
% Consider a finite sequence $\{X_k\}$ of independent, random, self-adjoint matrices that are positive-semidefinite (PSD) with $\lambda_{\max}\paren{X_k}\leq R$ almost surely (a.s) Compute the minimum and maximum eigenvalues of the sum of expectations,
% \[
% \mu_{\min}\coloneqq \lambda_{\min}\paren{\sum_{s=1}^m\E X_s} \quad, \quad \mu_{\max}\coloneqq \lambda_{\max}\paren{\sum_{s=1}^m\E X_s}
% \]
% Then,
% \begin{eqnarray} 
% \P\paren{\lambda_{\max}\paren{\sum_{s=1}^m X_s}\geq t\mu_{\max} } \leq m\brackets{\frac{e}{t}}^{t\mu_{\max}/R} ~~\forall t\geq e
% \end{eqnarray} 
% \end{lemma}
% As defined earlier, the initial weights are initialized iid with $W_{1,k}\sim \N(0,2/m)$. 
% %WLOG we will focus on $k=1$.
% Let $v_s\in \R^m$ be iid  Gaussian vectors $v_{s}\sim \N(0,m^{-1}I_{m})$. Define $X_{k,s}=v_sv_s^{\top}$, and notice that  $W_{1,k}^{\top}W_{1,k} \stackrel{\D}{=} \sum_{s=1}^m X_s$, and for $k_a=k_b+1: Z^i_{k_b+1, k_b}  \stackrel{\D}{=} 2D^i_{k_b+1}\paren{\sum_{s=1}^m X_{k,s}} D^i_{k_b}$. Furthermore, each $X_{k,s}$ is PSD of rank $\leq 1$ a.s, therefore $\lambda_{\max}\paren{X_{k,s}}=\sum_{r=1}^m \lambda_{r}\paren{X_{k,s}}=\Tr(X_{k,s})$. The trace of each matrix follows the conditional distribution of $m^{-1}\chi^2_{M}$ where $M=\nm{2D^i_{k_b+1}D^i_{k_b}}$. Since we are interested in an upper-bound for $Z^i_{k_b+1, k_b}$, we can increase the number of freedom degrees, 
% \[
% M=\nm{2D^i_{k_b+1}D^i_{k_b}}\leq 2\nm{D^i_{k_b}}\cdot 1, \textrm{~~and~~} \nm{D^i_{k_b}}\sim \textrm{Binom}(0.5,m)
% \]
% A corresponding concentration inequality for binomial variable,
% \[
% \P\paren{2\nm{D^i_{k_b}}\leq m \paren{1+\frac{\varepsilon}{L}}} \geq 1-\exp\left(-\frac{m\varepsilon^2}{L^2[4+2\varepsilon/3L]}\right) 
% \geq 1-\exp\left(-\frac{m\varepsilon^2}{5L^2}\right)   
% \]
% Therefore we can bound $\lambda_{\max}$ with high probability,
% %\paren{X_{k,s}}\sim m^{-1}\chi^2_{m(1+\frac{\varepsilon}{L})}$,
% \[
%     \Pr\left(\lambda_{\max}\paren{X_{k,s}} \leq \paren{1+\frac{\varepsilon}{L}}^2 \right) \geq 1-\exp\left(-\frac{m\varepsilon^2}{8L^2}\right)-\exp\left(-\frac{m\varepsilon^2}{5L^2}\right) \geq  1-2\exp\left(-\frac{m\varepsilon^2}{5L^2}\right)
% \]
% % % \[
% % % \P\paren{2\nm{D^i_{k_b}}\leq m \paren{1+\frac{\varepsilon}{L}}} \geq 1-\exp\left(-\frac{m\varepsilon^2}{L^2[4+2\varepsilon/3L]}\right) 
% % % \geq 1-\exp\left(-\frac{m\varepsilon^2}{5L^2}\right)   
% % % \]


% % $m^{-1}\nm{2D^i_{k_b+1}D^i_{k_b}}\chi^2_{m}$ for a given $\nm{2D^i_{k_b+1}D^i_{k_b}}$. Using $\chi^2$ concentration inequality, 
% % \[
% %     \Pr\left(\lambda_{\max}\paren{X_{k,s}} \in \brackets{\paren{1-\frac{\epsilon}{L}}\nm{2D^i_{k_b+1}D^i_{k_b}},\paren{1+\frac{\varepsilon}{L}}}\nm{2D^i_{k_b+1}D^i_{k_b}} \right) \geq 1-2\exp\left(-\frac{m\varepsilon^2}{8L^2}\right)
% % \]
% % As for the binary diagonal norm, $\nm{2D^i_{k_b+1}D^i_{k_b}}\leq 2\nm{D^i_{k_b}}\cdot 1$, and $\nm{D^i_{k_b}}\sim \textrm{Binom}(0.5,m)$, therefore,
% % \[
% % \P\paren{2\nm{D^i_{k_b}}\in \brackets{1-\frac{\epsilon}{L},1+\frac{\varepsilon}{L}}} \geq 
% % \]
% In addition,
% \[
% \mu_{\max}=\lambda_{\max}\paren{\E\brackets{ 2D^i_{k_b}\paren{\sum_{s=1}^m X_{k,s}}}}= \lambda_{\max}\paren{\frac{1}{m}\sum_{s=1}^m I_m}=1
% \]
% We are now ready to use lemma (\ref{lemma:tropp_2010}) with $\mu_{\max}=1, R=\paren{1+\frac{\varepsilon}{L}}^2$, and $t=e\log m$,
% \begin{eqnarray} 
% \P\paren{\nm{Z^i_{k_b+1, k_b}}\leq e\log m} \leq 1-2m\exp\left(-\frac{m\varepsilon^2}{8L^2}\right) -m\brackets{\log m}^{-\log m}
% \end{eqnarray} 
% We are now ready to use lemma (\ref{lemma:tropp_2010}) with $\mu_{\max}=1, R=\paren{1+\frac{\varepsilon}{L}}^2$, and $t=e\paren{1+\frac{\varepsilon}{L}}^2\log m$,
% \begin{eqnarray} 
% \P\paren{\nm{Z^i_{k_b+1, k_b}}\leq \paren{1+\frac{\varepsilon}{L}}^2e\log m} \leq 1-2m\exp\left(-\frac{m\varepsilon^2}{8L^2}\right) -m\brackets{\log m}^{-\log m}
% \end{eqnarray} 
% The inductive step will follow the same argument. Given a series,
% \begin{eqnarray*} 
% &&\lambda_{\max}\paren{\brackets{W_{k_b} D^i_{k_b}\ldots W_{k_a} D^i_{k_a}}^{\top}\brackets{W_{k_b} D^i_{k_b}\ldots W_{k_a} D^i_{k_a}}} \\ 
% &\leq& \lambda_{\max}\paren{W_{k_a} D^i_{k_a} \brackets{D^i_{k_a}}^{\top} \brackets{W_{k_a}}^{\top} } \lambda_{\max}\paren{\brackets{W_{k_b} D^i_{k_b}\ldots W_{k_a-1} D^i_{k_a-1}}^{\top}\brackets{W_{k_b} D^i_{k_b}\ldots W_{k_a-1} D^i_{k_a-1}}} \\
% &\leq& \ldots \leq \paren{1+\frac{\varepsilon}{L}}^{2(k_a-k_b)}\leq e^{2\varepsilon} \quad \textrm{with probability larger than~~} 1-2L^2\exp\left(-\frac{m\varepsilon^2}{5L^2}\right).
% \end{eqnarray*} 
% Where we used the invariance of eigenvalues under cyclic permutation, and the submultiplicativity of symmetric and (a.s) positive definite matrices. 
% As for $\mu_{\max}$,
% \[
% \mu_{\max}=\lambda_{\max}\paren{\E\brackets{\brackets{W_{k_b} D^i_{k_b}\ldots W_{k_a} D^i_{k_a}}^{\top}\brackets{W_{k_b} D^i_{k_b}\ldots W_{k_a} D^i_{k_a}}} }=1
% \]
% Due to statistical Independence. We can now reuse lemma (\ref{lemma:tropp_2010}) for general $k_a,k_b$ with $\mu_{\max}=1, R=e^{2\varepsilon}$, and $t=e^{2\varepsilon}\log m$,
% \begin{eqnarray*} 
% \P\paren{\nm{Z^i_{k_a, k_b}}\leq e^{2\varepsilon}\log m} \leq 1-mL^2\paren{2\exp\left(-\frac{m\varepsilon^2}{8L^2}\right) +\brackets{e^{2\varepsilon-1}\log m}^{-\log m}}
% \end{eqnarray*} 
% \end{proof}


% \asaf{new proof for leamma 6:}
% \begin{proof}
% We start with a bound to the spectral norm of a sum of independent random matrices,
% \begin{lemma}[Matrix Chernoff bound, \cite{tropp2012user} Remark $5.3$] \label{lemma:tropp_2010}
% Consider a finite sequence $\{X_k\}$ of independent, random, self-adjoint matrices that are positive-semidefinite (PSD) with $\lambda_{\max}\paren{X_k}\leq R$ almost surely (a.s) Compute the minimum and maximum eigenvalues of the sum of expectations,
% \[
% \mu_{\min}\coloneqq \lambda_{\min}\paren{\sum_{s=1}^m\E X_s} \quad, \quad \mu_{\max}\coloneqq \lambda_{\max}\paren{\sum_{s=1}^m\E X_s}
% \]
% Then,
% \begin{eqnarray} 
% \P\paren{\lambda_{\max}\paren{\sum_{s=1}^m X_s}\geq t\mu_{\max} } \leq m\brackets{\frac{e}{t}}^{t\mu_{\max}/R} ~~\forall t\geq e
% \end{eqnarray} 
% \end{lemma}

% We will proof first the upper bound by induction. Fix $k_a=k_b+1$, so  $Z^i_{k_b+1, k_b}=D^{i}_{k_b+1} W_{1,k_b}D^i_{k_b}$, and 
% $\nm{Z^i_{k_b+1, k_b}}\leq \nm{W_{1,k_b}D^{i}_{k_b+1}}$. 
% As the columns of $W_{1,k_b}$ are independent, we have $W\vcentcolon= W_{1,k_b}D^{i}_{k_b+1}= \brackets{w_1d_{1,1},\ldots,w_m d_{m,m}}$ 
% where $w_s$ is the $s$th column of $W_{1,k_b}$ and $d$'s are independent Bernoulli random variables with $p=0.5$. We now split $\brackets{m}$ into $r=\left \lceil{\paren{1+\frac{\varepsilon}{L}}^2\log m}\right \rceil  $ intervals, so the $l$th interval contains $S^l=\braces{\frac{m(l-1)}{r}+1,\ldots,\frac{ml}{r}}$, and the matrix $W^l$ has the corresponding columns of $W$, with the rest replaced with zeros. Therefore,
% \[
% \nm{W}=\nm{\sum_{l=1}^{r}W^l}\leq \sum_{l=1}^{r}\nm{W^l}\leq r \max\limits_{l}\nm{W^l}
% \]
% For a fixed $l$ we can derive,
% \[
% \brackets{W^l}^{\top}W^l=\sum_{s=1}^m v_s^l\brackets{v_s^l}^{\top}=\sum_{s=1}^m \tilde{v}_s^l\brackets{\tilde{v}_s^l}^{\top}
% \]
% Where $v_s^l$ is the $s$th row of $W^l$, and $\tilde{v}_s^l$ is its subset of $S^l$ indices. 
% Define $X_s=\tilde{v}_s^l\brackets{\tilde{v}_s^l}^{\top}$, each $X_{s}$ is PSD of maximal rank $1$, therefore $\lambda_{\max}\paren{X_{s}}=\Tr(X_{s})$. The trace of each matrix follows the conditional distribution of 
% $m^{-1}\chi^2_{M}$ where $M=2\sum_{s\in S^l}d_{s,s}$. Fix $\varepsilon<1$, we have,
% \begin{eqnarray*}
% \Pr\left( m^{-1}\chi^2_{M} \geq \frac{1}{\log m}\paren{1+\frac{\varepsilon}{L}}^2 \right) &\leq& \Pr\left( M> 1+\frac{\varepsilon}{L}\right) + \Pr\left(m^{-1}\chi^2_{M} \geq \frac{1}{\log m}\paren{1+\frac{\varepsilon}{L}}^2  | M=1+\frac{\varepsilon}{L}    \right) \\
% &\leq& \exp\left(-\frac{m\varepsilon^2}{L^2\log m[4+2\varepsilon/3L]}\right) + \exp\left(-\frac{m\varepsilon^2}{8L^2\log m}\right) \\ 
% &\leq& 2\exp\left(-\frac{m\varepsilon^2}{5L^2\log m}\right)
% \end{eqnarray*}
% \begin{eqnarray*}
% \Pr\left( m^{-1}\chi^2_{M} \geq \frac{1}{\log m} \right) &\leq& \Pr\left( M> \frac{m}{\log m (1+\frac{\varepsilon}{L})}\right) + \Pr\left(m^{-1}\chi^2_{M} \geq \frac{1}{\log m}| M=\frac{m}{\log m (1+\frac{\varepsilon}{L})}    \right) \\
% &\leq& \exp\left(-\frac{m\varepsilon^2}{2L^2\log m[1+\varepsilon/3L][1+\frac{\varepsilon}{L}]}\right) + \exp\left(-\frac{m\varepsilon^2}{8L^2\log m \paren{1+\frac{\varepsilon}{L}}^2}\right) \\ 
% &\leq& 2\exp\left(-\frac{m\varepsilon^2}{8L^2\log m \paren{1+\frac{\varepsilon}{L}}^2}\right)
% \end{eqnarray*}
% So with a high probability $\lambda_{\max}\paren{X_{s}}\leq \frac{1}{\log m}$. As for $\mu_{\max}$,
% \[
% \mu_{\max}=\lambda_{\max}\paren{\E\brackets{ 2D^i_{k_b}\paren{\sum_{s=1}^m X_{s}}}}= \lambda_{\max}\paren{\frac{1}{m}\sum_{s=1}^m I_m}=1
% \]
% We are now ready to use lemma (\ref{lemma:tropp_2010}) with $\mu_{\max}=1, R=\frac{1}{\log m}$, and $t>e$,
% \begin{eqnarray} 
% \P\paren{\nm{Z^i_{k_b+1, k_b}}^2\leq t} \leq 1-2m\exp\left(-\frac{m\varepsilon^2}{8L^2\log m \paren{1+\frac{\varepsilon}{L}}^2}\right) -m\paren{\frac{t}{e}}^{-t\log m}
% \end{eqnarray} 


% \newpage
% \asaf{old:}
% As defined earlier, the initial weights are initialized iid with $W_{1,k}\sim \N(0,2/m)$. 
% %WLOG we will focus on $k=1$.
% Let $v_s\in \R^m$ be iid  Gaussian vectors $v_{s}\sim \N(0,m^{-1}I_{m})$. Define $X_{k,s}=v_sv_s^{\top}$, and notice that  $W_{1,k}^{\top}W_{1,k} \stackrel{\D}{=} \sum_{s=1}^m X_s$, and for $k_a=k_b+1: Z^i_{k_b+1, k_b}  \stackrel{\D}{=} 2D^i_{k_b+1}\paren{\sum_{s=1}^m X_{k,s}} D^i_{k_b}$. Furthermore, each $X_{k,s}$ is PSD of rank $\leq 1$ a.s, therefore $\lambda_{\max}\paren{X_{k,s}}=\sum_{r=1}^m \lambda_{r}\paren{X_{k,s}}=\Tr(X_{k,s})$. The trace of each matrix follows the conditional distribution of $m^{-1}\chi^2_{M}$ where $M=\nm{2D^i_{k_b+1}D^i_{k_b}}$. Since we are interested in an upper-bound for $Z^i_{k_b+1, k_b}$, we can increase the number of freedom degrees, 
% \[
% M=\nm{2D^i_{k_b+1}D^i_{k_b}}\leq 2\nm{D^i_{k_b}}\cdot 1, \textrm{~~and~~} \nm{D^i_{k_b}}\sim \textrm{Binom}(0.5,m)
% \]
% A corresponding concentration inequality for binomial variable,
% \[
% \P\paren{2\nm{D^i_{k_b}}\leq m \paren{1+\frac{\varepsilon}{L}}} \geq 1-\exp\left(-\frac{m\varepsilon^2}{L^2[4+2\varepsilon/3L]}\right) 
% \geq 1-\exp\left(-\frac{m\varepsilon^2}{5L^2}\right)   
% \]
% Therefore we can bound $\lambda_{\max}$ with high probability,
% %\paren{X_{k,s}}\sim m^{-1}\chi^2_{m(1+\frac{\varepsilon}{L})}$,
% \[
%     \Pr\left(\lambda_{\max}\paren{X_{k,s}} \leq \paren{1+\frac{\varepsilon}{L}}^2 \right) \geq 1-\exp\left(-\frac{m\varepsilon^2}{8L^2}\right)-\exp\left(-\frac{m\varepsilon^2}{5L^2}\right) \geq  1-2\exp\left(-\frac{m\varepsilon^2}{5L^2}\right)
% \]
% % % \[
% % % \P\paren{2\nm{D^i_{k_b}}\leq m \paren{1+\frac{\varepsilon}{L}}} \geq 1-\exp\left(-\frac{m\varepsilon^2}{L^2[4+2\varepsilon/3L]}\right) 
% % % \geq 1-\exp\left(-\frac{m\varepsilon^2}{5L^2}\right)   
% % % \]


% % $m^{-1}\nm{2D^i_{k_b+1}D^i_{k_b}}\chi^2_{m}$ for a given $\nm{2D^i_{k_b+1}D^i_{k_b}}$. Using $\chi^2$ concentration inequality, 
% % \[
% %     \Pr\left(\lambda_{\max}\paren{X_{k,s}} \in \brackets{\paren{1-\frac{\epsilon}{L}}\nm{2D^i_{k_b+1}D^i_{k_b}},\paren{1+\frac{\varepsilon}{L}}}\nm{2D^i_{k_b+1}D^i_{k_b}} \right) \geq 1-2\exp\left(-\frac{m\varepsilon^2}{8L^2}\right)
% % \]
% % As for the binary diagonal norm, $\nm{2D^i_{k_b+1}D^i_{k_b}}\leq 2\nm{D^i_{k_b}}\cdot 1$, and $\nm{D^i_{k_b}}\sim \textrm{Binom}(0.5,m)$, therefore,
% % \[
% % \P\paren{2\nm{D^i_{k_b}}\in \brackets{1-\frac{\epsilon}{L},1+\frac{\varepsilon}{L}}} \geq 
% % \]
% In addition,
% \[
% \mu_{\max}=\lambda_{\max}\paren{\E\brackets{ 2D^i_{k_b}\paren{\sum_{s=1}^m X_{k,s}}}}= \lambda_{\max}\paren{\frac{1}{m}\sum_{s=1}^m I_m}=1
% \]
% We are now ready to use lemma (\ref{lemma:tropp_2010}) with $\mu_{\max}=1, R=\paren{1+\frac{\varepsilon}{L}}^2$, and $t=e\log m$,
% \begin{eqnarray} 
% \P\paren{\nm{Z^i_{k_b+1, k_b}}\leq e\log m} \leq 1-2m\exp\left(-\frac{m\varepsilon^2}{8L^2}\right) -m\brackets{\log m}^{-\log m}
% \end{eqnarray} 
% We are now ready to use lemma (\ref{lemma:tropp_2010}) with $\mu_{\max}=1, R=\paren{1+\frac{\varepsilon}{L}}^2$, and $t=e\paren{1+\frac{\varepsilon}{L}}^2\log m$,
% \begin{eqnarray} 
% \P\paren{\nm{Z^i_{k_b+1, k_b}}\leq \paren{1+\frac{\varepsilon}{L}}^2e\log m} \leq 1-2m\exp\left(-\frac{m\varepsilon^2}{8L^2}\right) -m\brackets{\log m}^{-\log m}
% \end{eqnarray} 
% The inductive step will follow the same argument. Given a series,
% \begin{eqnarray*} 
% &&\lambda_{\max}\paren{\brackets{W_{k_b} D^i_{k_b}\ldots W_{k_a} D^i_{k_a}}^{\top}\brackets{W_{k_b} D^i_{k_b}\ldots W_{k_a} D^i_{k_a}}} \\ 
% &\leq& \lambda_{\max}\paren{W_{k_a} D^i_{k_a} \brackets{D^i_{k_a}}^{\top} \brackets{W_{k_a}}^{\top} } \lambda_{\max}\paren{\brackets{W_{k_b} D^i_{k_b}\ldots W_{k_a-1} D^i_{k_a-1}}^{\top}\brackets{W_{k_b} D^i_{k_b}\ldots W_{k_a-1} D^i_{k_a-1}}} \\
% &\leq& \ldots \leq \paren{1+\frac{\varepsilon}{L}}^{2(k_a-k_b)}\leq e^{2\varepsilon} \quad \textrm{with probability larger than~~} 1-2L^2\exp\left(-\frac{m\varepsilon^2}{5L^2}\right).
% \end{eqnarray*} 
% Where we used the invariance of eigenvalues under cyclic permutation, and the submultiplicativity of symmetric and (a.s) positive definite matrices. 
% As for $\mu_{\max}$,
% \[
% \]
% Due to statistical Independence. We can now reuse lemma (\ref{lemma:tropp_2010}) for general $k_a,k_b$ with $\mu_{\max}=1, R=e^{2\varepsilon}$, and $t=e^{2\varepsilon}\log m$,
% \begin{eqnarray*} 
% \P\paren{\nm{Z^i_{k_a, k_b}}\leq e^{2\varepsilon}\log m} \leq 1-mL^2\paren{2\exp\left(-\frac{m\varepsilon^2}{8L^2}\right) +\brackets{e^{2\varepsilon-1}\log m}^{-\log m}}
% \end{eqnarray*} 
% \end{proof}
% \newpage
\begin{lemma} \label{lemma:tao_bound}
The maximal variation defined in~(\ref{def:tau}) satisfies:$\quad \tau \leq \frac{8\sqrt{3\ell(W_1)}\beta}{\alpha^2L }$.
\end{lemma}
\begin{proof}
Lemma~\ref{lemma:linear_rate} bounds $\nm{\nabla_k\ell(W_t)}_2$ based on assumption~(\ref{eqn:gamma-upper-bound}),  which hold with probability of at least $1 - \exp(-\Omega(\sqrt{m}))$ as assured by theorem~\ref{thm:bound_gamma}. therefore,
%We thus need to bound $\tau$,
\begin{eqnarray*} \label{eqn:tau_val}
\tau = \max\limits_{1 \leq t \leq T}\max\limits_{k\in [L]} \nm{W_{t,k}-W_{1,k}}_2 &\leq& \sum_{t=1}^{T-1}\max\limits_{k\in [L]} \nm{W_{t+1,k}-W_{t,k}}_2 \\
&=& \eta\sum_{t=1}^{T-1}\max\limits_{k\in [L]} \nm{\nabla_k\ell(W_t)}_2 \\
&\leq& \sqrt{3}\eta\beta\sum_{t=1}^{T-1}\sqrt{\ell(W_t)} \\
&\leq& \sqrt{3\ell(W_1)}\eta\beta\sum_{t=0}^{T-1}\left(1-\frac{\eta\alpha^2 L}{4}\right)^{\frac{t}{2}} \\
&\leq& \frac{8\sqrt{3\ell(W_1)}\beta}{\alpha^2L }
\end{eqnarray*}
with probability of at least $1 - \exp(-\Omega(\sqrt{m}))$, where in the last transition we used, $0<x<1: \sqrt{1-x}<1-x/2$.
\end{proof}

\section{Detailed Proofs}
\subsection{Proof for Lemma~\ref{lemma:linear_rate}}
\begin{proof} \label{proof:lemma_linear_rate}
Using the assumption in (\ref{eqn:eig-lower-bound}), (\ref{eqn:eig-upper-bound}), (\ref{eqn:cross-upper-bound}) and (\ref{eqn:gamma-upper-bound}), by setting $a_i = \frac{\beta^4L^2}{m}$, we have
\[
    \Lambda_i + \eta^2 a_i \leq -2\eta\frac{\alpha^2 L}{m} + 2\eta\frac{\beta^2\gamma nL}{m} + 4\eta^2\frac{\beta^4L^2}{m^2} + 3\eta^2\frac{\beta^4\gamma^2n^2L^2}{m^2} \leq -\eta\frac{\alpha^2 L}{m} + 6\eta^2\frac{\beta^4L^2}{m^2}
\]
By choosing step size $\eta$ as
\begin{eqnarray}
    \eta \leq \frac{\min(1, \alpha^2)m}{12\beta^4 L} \label{eqn:eta-bound}
\end{eqnarray}
we have
\[
    \Lambda_i + \eta^2 a_i \leq -\frac{\eta\alpha^2 L}{2m}
\]
and therefore
\[
    \ell(W_{t+1}) - \ell(W_t) \leq -\frac{\eta\alpha^2 L}{2m}\ell(W_t) + \frac{\eta^2}{\beta^4L^2}\sum_{i=1}^n \nm{\Delta_{t,i}x_i}^2
\]
%\asaf{recheck the $2$ constants, might be $4$}
Next, we need to bound $\nm{\Delta_{t,i}x_i}^2$. To this end, we first bound $\nm{\nabla_k\ell(W_t)}_2$
\begin{eqnarray*}
\lefteqn{\langle\nabla_k\ell(W_t), \nabla_k\ell(W_t)\rangle} \\
& \leq & \sum_{i=1}^n \mbox{vec}^{\top}\left((W_t^i - \Phi_i)x_ix_i^{\top}\right)\left(F_{t,k+1}^i\left[F_{t,k+1}^i\right]^{\top}\otimes \left[G_{t,k-1}^i\right]^{\top}G_{t,k-1}^i\right)\mbox{vec}\left((W_t^i - \Phi_i)x_ix_i^{\top}\right) \\
&  & + \sum_{i=1}^n \sum_{i\neq j} \left[G_{t,k-1}^ix_i\right]^{\top}G_{t,k-1}^jx_j \left\langle \left[F_{t,k+1}^i\right]^{\top}(W_t^i - \Phi_i)x_i, \left[F_{t,k+1}^j\right]^{\top}(W_t^j - \Phi_j)x_j\right\rangle \\
& \leq & \sum_{i=1}^n \left\|F_{t,k+1}^i\left[F_{t,k+1}^i\right]\right\|\left\|\left[G_{t,k-1}^i\right]^{\top}G_{t,k-1}^i\right\|\|(w_t^i - \Phi_i)x_i\|^2 \\
&     & + \sum_{i=1}^n\left[G^i_{t,k-1}x_i\right]^{\top}G^j_{t,k-1}x_j
\left\|F_{t,k+1}^jF_{t,k+1}^i\right\|_2\left|(w_t^i - \Phi_i)x_i\right|\left|(w_t^j - \Phi_j)x_j\right| \\
& \leq & 2\left(\beta^2 + n\gamma\beta^2\right)\ell(W_t) \leq \frac{3\beta^2}{m}\ell(W_t)
\end{eqnarray*}
Where~(\ref{eqn:gamma-upper-bound}) was used in the last transition. We can rewrite $\Delta_{t,i}$ as
\begin{eqnarray*}
\Delta_{t,i} = \sum_{s=2}^L(-\eta)^{s-2}\sum_{k_1 > k_2>\ldots>k_s} F_{t,k_1+1}^i\left(\prod_{\ell=1}^s \nabla_{k_{\ell}}\ell(W_t)Z^i_{k_{\ell}-1,k_{\ell-1}}\right)G^i_{t,k_s-1}
\end{eqnarray*}
and therefore, according to Lemma~\ref{lemma:z-ka-kb-t}, for any $\epsilon \in (0, 1/5)$,  with a probability $1 - L^2\sqrt{m}\exp\left(-\epsilon m/[4L] + 6\sqrt{m}\right)$
\asaf{change $Z$ term to the upper log-bound.}
\[
\|\Delta_{t,i}\|_2 \leq \sum_{s=2}^L \beta\eta^{s-2}\left(5\sqrt{3}e^{\epsilon/2}m^{1/4}L\beta\sqrt{\ell(w_t)}\right)^s \leq \frac{75e^{\epsilon}\sqrt{m}L^2\beta^3\ell(W_t)}{1 - 5\sqrt{3}e^{\epsilon/2}\eta m^{1/4}L\beta\sqrt{\ell(W_1)}}
\]
Where $\binom{L}{s}< L^s$ and $\ell(w_t) \leq \ell(w_1)$ were used, and therefore,
\asaf{change $Z$ term to the upper log-bound.}
% where the last step follows $\ell(w_t) \leq \ell(w_1)$, and therefore
\[
    \ell(W_{t+1}) - \ell(W_t) \leq -\frac{\eta\alpha^2 L}{2}\ell(W_t) + \frac{75^2e^{\epsilon}\eta^2m\beta^2 L^2n\ell^2(W_t)}{1 - 5\sqrt{3}e^{\epsilon/2}\eta m^{1/4}L\beta\sqrt{\ell(W_1)}}
\]
\end{proof}

\subsection{Proof for Theorem~\ref{thm:bound_alpha_beta}}
\begin{proof} \label{proof:thm_bound_alpha_beta}
We will focus on $G^i_{t,k}$ first and similar analysis will be applied to $F^i_{t,k}$. To bound $\nm{\left[G^i_{t,k}\right]^{\top}G^i_{t,k}}_2$, we will bound $\max\limits_{\nm{v} \leq 1} \nm{G^i_{t,k}v}^2$. We expand $G^i_{t,k}$ as
\begin{eqnarray*}
    \lefteqn{G^i_{t,k} = D^i_k\left(W_{1,k} + \delta W_{t,k}\right)\ldots D^i_1\left(W_{1,1} + \delta W_{t,1}\right)D_0^iC = D^i_kW_{1,k}\ldots D^i_0C} \\
    & + & \sum_{s=1}^k \sum_{k_1 > k_2 > \ldots > k_s} D^i_kW_{1,k}\ldots D^i_{k_1}\delta W_{t,k_1}D^i_{k_1-1}W_{1,k_1-1}\ldots D^i_{k_s}\delta W_{t,k_s}D^i_{k_s-1}W_{1,k_s-1}\ldots D^i_0C
\end{eqnarray*}
Where $\delta W_{t,k}=W_{t,k}-W{1,k}$. Define $Z_{k_a, k_b} = D_{k_a}^iW_{1,k_a}\ldots W_{1,k_b+1}D_{k_b}^i$ and $k_0 = k$, therefore,
\[
    G_{t,k}^i = Z_{k,0}C + \sum_{s=1}^k \sum_{k_1 > k_2>\ldots>k_s} \left(\prod_{j=1}^{s} Z_{k_{j-1}, k_j}\delta W_{t,k_j}\right)Z_{k_s-1,0}C
\]
According to Lemma~\ref{lemma:z-ka-kb}, we have, with a probability $1 - L^2\sqrt{m}\exp\left(-\epsilon m/[4L] + 6\sqrt{m}\right)$, for any $1 \leq k_b \leq k_a \leq L$ and any $\epsilon \in (0,1/5)$,
\asaf{change based in lemma \ref{lemma:z-ka-kb}}
\[
    \|Z_{k_a, k_b}\|_2 \in\left[m^{1/4}e^{-\epsilon}, \sqrt{3}m^{1/4}e^{\epsilon/2}\right]
\]
Following the same analysis as in Lemma~\ref{lemma:z-ka-kb}, we have, with a probability $ 1- 2L^2\exp(-\epsilon m/[4L] +3d_x)$, we have
\[
\min\limits_{u \in \R^d}\frac{\nm{Z_{k_a, k_b} C u}}{\nm{u}} \geq \sqrt{\frac{m}{3d_x}}e^{-\epsilon}
\]
and
\[
\max\limits_{u \in \R^d}\frac{\nm{Z_{k_a, k_b} C u}}{\nm{u}} \geq \sqrt{\frac{3m}{d_x}}e^{\epsilon/2}
\]
Combining the above results together, we have, with a probability $ 1- 3L^2\sqrt{m}\exp(-\epsilon m/[4L] + 6\sqrt{m}+3d_x)$,
\[
\min\limits_{u \in \R^{d_x}}\frac{\nm{G_{t,k}^iu}}{\nm{u}} \geq \sqrt{\frac{m}{3d_x}}e^{-\epsilon} - \sqrt{\frac{3m}{d_x}}e^{\epsilon/2}\sum_{s=1}^L L^s \left(\sqrt{3}\tau m^{1/4}e^{\epsilon/2}\right)^s \geq  \sqrt{\frac{m}{3d_x}}e^{-\epsilon}\left(1 - \frac{3\sqrt{3}e^{2\epsilon}m^{1/4}L\tau}{1 - \sqrt{3}m^{1/4}e^{\epsilon/2}L\tau}\right)
\]
and
\[
\max\limits_{u \in \R^{d_x}}\frac{\nm{G_{t,k}^i u}}{\nm{u}} \leq \sqrt{\frac{3m}{d_x}}e^{\epsilon/2} + \sqrt{\frac{3m}{d_x}}e^{\epsilon/2}\sum_{s=1}^L L^s \left(\sqrt{3}\tau m^{1/4}e^{\epsilon/2}\right)^s \leq \sqrt{\frac{3m}{d_x}}e^{\epsilon/2}\left(1 + \frac{\sqrt{3}e^{\epsilon/2}m^{1/4}L\tau}{1 - \sqrt{3}m^{1/4}e^{\epsilon/2}L\tau}\right)
\]
Since
\[
    \sqrt{3}e^{2\epsilon}m^{1/4}L\tau \leq \frac{1}{9}
\]
we have, with a probability $ 1- 3L^2\sqrt{m}\exp(-\epsilon m/[4L] + 6\sqrt{m}+3d_x)$,
\[
\min\limits_{u \in \R^{d_x}}\frac{\nm{G_{t,k}^iu}_2}{\nm{u}} \geq \frac{1}{2}\sqrt{\frac{m}{3d_x}}, \quad \max\limits_{u \in \R^{d_x}}\frac{\nm{G_{t,k}^iu}}{\nm{u}} \leq \frac{3}{2}\sqrt{\frac{3m}{d_x}}
\]
The same analysis applies to $\nm{F_{t,k}^i}_2$, with corresponding initialization variance of $(m d_y)^{-1}$
\end{proof}


\subsection{Proof for Theorem~\ref{thm:bound_gamma}}
\begin{proof} \label{proof:thm_bound_gamma}
To bound $\nm{F_{t,k}^j\left[F_{t,k}^i\right]^{\top}}_2$, we define $k_0 = L+1$ and 
\[
    Z^j_{k_a:k_b} = D_{k_a}^jW_{1,k_a}D_{k_a - 1}^jW_{1,k_a - 1}\ldots W_{1,k_b+1}D^j_{k_b}
\]
and express $F_{t,k}^j\left[F_{t,k}^i\right]^{\top}$ as
\begin{eqnarray*}
\lefteqn{F_{t,k}^j\left[F_{t,k}^i\right]^{\top}} \\
& = & \underbrace{BD^j_LW_{1,L}\ldots W_{1,k+1} D^j_kD_k^iW_{1,k+1}^{\top}\ldots W_{1,L}^{\top}D^i_LB^{\top}}_{:=Z} \\
&   & + \underbrace{BZ_{L:k}^j\sum_{s=1}^{L-k} \left[\left(\prod_{\ell=1}^{s}Z_{k_{\ell-1}-1:k_{\ell}}^{i}\delta W_{t,k_{\ell}}\right) Z^i_{k_{s}-1:k}\right]^{\top}B^{\top}}_{:=\A_1} + \underbrace{B\sum_{s=1}^{L-k} \left[\left(\prod_{\ell=1}^{s}Z_{k_{\ell-1}-1:k_{\ell}}^{j}\delta W_{t,k_{\ell}}\right)Z^j_{k_{s}-1:k}\right]\left[Z_{L:k}^i\right]^{\top} B^{\top}}_{:=\A_2} \\
&   & + \underbrace{B\sum_{s_a=1}^{L-k}\sum_{s_b=1}^{L-k} \left(\prod_{\ell=1}^{s_a}Z_{k_{\ell-1}:k_{\ell}}^{j}\delta W_{t,k_{\ell}}\right)Z^j_{k_{s_a}-1:k}\left[Z^i_{k_b-1:k}\right]^{\top}\left[\prod_{\ell=2}^{s_b}Z_{k_{\ell-1}:k_{\ell}}^{i}\delta W_{t,k_{\ell}}\right]^{\top}B^{\top}}_{:=\A_3}
\end{eqnarray*}
According to Lemma~\ref{lemma:z-ka-kb}, with a probability $1 - 3L^2\sqrt{m}\exp\left(-\epsilon m/[4L] + 6\sqrt{m} + 3d\right)$,
\asaf{change left term based on lemma \ref{lemma:z-ka-kb}:}
\[
    \|Z_{k_a, k_b}\|_2 \leq \sqrt{3}e^{\epsilon/2}m^{1/4}, \quad \max\limits_{\|v\| \leq 1} \left\|v^{\top}BZ_{k_a,k_b} \right\| \leq \frac{3}{2}\sqrt{\frac{3m}{d}}
\]
As a result, with a probability $1 - 3L^2\sqrt{m}\exp\left(-\epsilon m/[4L] + 6\sqrt{m} + 3d\right)$, we have
\begin{eqnarray*}
\max\limits_{|v| \leq 1} v^{\top}\A_1 v \leq \frac{27m}{4d}\sum_{s=1}^L \left(\sqrt{3}e^{\epsilon/2}m^{1/4}L\tau\right)^s \leq \xi \frac{m}{d}
\end{eqnarray*}
where $\xi = 5\sqrt{3}e^{\epsilon/2}m^{1/4}L\tau \ll 1$ and the last step utilizes the assumption $\sqrt{3}e^{\epsilon/2}m^{1/4}L\tau \leq 1/9$.
Using the same analysis, we have, with a probability $1 - 3L^2\exp(-\epsilon m/L + 6\sqrt{m} + 3d)$,
\[
    \max\limits_{|v| \leq 1} v^{\top}\A_2v \leq \xi\frac{m}{d}, \quad \max\limits_{|v| \leq 1} v^{\top}\A_3v \leq \xi^2\frac{m}{d}
\]
What's left is to bound the spectral norm of $Z = F_{1,k}^j\left[F_{1,k}^i\right]$. To this end, we will bound
\[
    \max\limits_{u\in \R^d, v\in \R^d, |u| =1, |v| = 1} \left\langle \left[F^j_{1,k}\right]^{\top}u, \left[F^i_{1,k}\right]^{\top}v\right\rangle
\]
Define
\[
    a_k = \left[F^j_{t,k+1}\right]u, \quad b_k = \left[F^i_{t,k+1}\right]u
\]
We have
\begin{eqnarray}
\lefteqn{a^{\top}_{k} b_{k} = a_{k+1}^{\top}W_{1,k+1}D_k^j D_k^i W^{\top}_{1,k+1} b_{k+1}} \nonumber \\
& = & \underbrace{a_{k+1}^{\top}W_{1,k+1}D_k^j D_k^i W^{\top}_{1,k+1} P_{a_{k+1}}\left(b_{k+1}\right)}_{:=Z_1} + \underbrace{a_{k+1}^{\top}W_{1,k+1}D_k^j D_k^i W^{\top}_{1,k+1}\left(b_{k+1} - P_{a_{k+1}}\left(b_{k+1}\right)\right)}_{:=Z_2} \nonumber
\end{eqnarray}
where $P_a(b) = aa^{\top}b/\nm{a}^2$ projects vector $b$ onto the direction of $a$. Since $W^{\top}_{1,k+1}\left(b_{k+1} - P_{a_{k+1}}(b_{k+1})\right)$ is statistically independent from $W_{1,k+1}^{\top}a_{k+1}$, by fixing $W_{1,k+1}^{\top}a_{k+1}$ and viewing $Z_2$ as a random variable of $W^{\top}_{1,k+1}\left(b_{k+1} - P_{a_{k+1}}(b_{k+1})\right)$, we have $Z_2$ follow $\N(0, \sigma^2)$ distribution, where
\[
    \sigma^2 = \frac{1}{m}\nm{b_{k+1} - P_{a_{k+1}}(b_{k+1})}^2\nm{D_k^jW_{1,k+1}^{\top}a_{k+1}}^2
\]
Using the property of Gaussian distribution, we have, with a probability $1 - 2\exp(-\sqrt{m}/2)$,
\asaf{I think $m^{0.25}$ should be replaced with a constant:}
\[
\left|Z_2\right| \leq \frac{\nm{b_{k+1}}}{m^{1/4}}\nm{D_k^jW_{1,k+1}^{\top}a_{k+1}}
\]
Since $\nm{D_k^jW_{1,k+1}^{\top}a_{k+1}}^2$ follows $2|a_{k+1}|^2/m\chi^2_{m/2}$, with a probability $1 - \exp(-\epsilon m/4)$, we have
\[
\nm{D_k^jW_{1,k+1}^{\top}a_{k+1}}^2 \leq (1 + \epsilon)\nm{a_{k+1}}^2
\]
Combining the above two results, with a probability $1 - 2\exp(-\sqrt{m}/2) - \exp(-\epsilon m/4)$,
\[
\left|Z_2\right| \leq \frac{1+\epsilon}{m^{1/4}}\nm{b_{k+1}}\nm{a_{k+1}} \leq \frac{(1+\epsilon)\beta}{m^{1/4}}
\]
where the last step utilizes the fact $\nm{b_{k+1}} \leq \sqrt{\beta}$ and $\nm{a_{k+1}} \leq \sqrt{\beta}$.

To bound $Z_1$, let $\I_k^{i,j}$ be the set of indices of diagonal elements that are nonzero in both $D_k^j$ and $D_k^i$. According to Lemma~\ref{lemma:1}, with a probability $1 - \exp(-\Omega(m))$, we have $|\I_k^{i,j}| \leq m/3$. Define $u = W^{\top}_{1,k+1}a_{k+1}/\nm{a_{k+1}}$. We have
\[
    Z_1 \leq \left|a_{k+1}^{\top}b_{k+1}\right|\sum_{s \in \I_k^{i,j}} u_s^2 
\]
%\asaf{Duplication.Equals or leq here?}
Using the concentration of $\chi^2$ distribution, we have, with a probability $1 - \exp(-\epsilon m/3))$
\[
\sum_{s \in \I_k^{i,j}} u_i^2 \leq \frac{2(1+\epsilon)}{3}
\]
By combining the results for $Z_1$ and $Z_2$, for a fixed normalized $u\in \R^d$, $v \in R^d$, with a probability $1 - \exp(-\Omega(\sqrt{m})$, we have
\[
    \left|\left\langle\left[F_{1,k}^j\right]^{\top}u, \left[F_{1,k}^i\right]^{\top}v\right\rangle\right| \leq \frac{(1+\epsilon)\beta}{m^{1/4}} + \frac{2(1+\epsilon)}{3}\left|\left\langle\left[F_{1,k+1}^j\right]^{\top}u, \left[F_{1,k+1}^i\right]^{\top}v\right\rangle\right|
\]
By combining the results over iterations, we have, with a probability $1 - 2L\exp(-\epsilon m/3) - 2L\exp\left(-\sqrt{m}/2\right)$, for fixed normalized $u \in \R^d$ and $v \in R^d$
\[
\left|\left\langle\left[F_{t,k}^j\right]^{\top}u, \left[F_{t,k}^i\right]^{\top}v\right\rangle\right| \leq \frac{4(1+\epsilon)\beta}{m^{1/4}} + \left(\frac{2(1+\epsilon)}{3}\right)^{L-k}\beta
\]
We extend the result to any $u$ and $v$ by using the theory of covering number, and complete the proof by choosing $\epsilon = 1/6$.

To bound $|\langle G_{t,k}^j x_j, G_{t,k} x_i\rangle|$, follow the same analysis in above, we have
\[
\left|\langle G_{t,k}^j x_j, G^i_{t,k} x_i\rangle\right| \leq O\left(m^{1/4}L\tau\beta\right) + \left|\langle G_{1,k}^j x_j, G^i_{1,k} x_i\rangle\right| \leq O\left(\left(m^{1/4}L\tau + \frac{1}{m^{1/4}}\right)\beta\right) + \left(\frac{5}{6}\right)^{k}\langle Cx_i, Cx_j\rangle
\]
We expand $\langle Cx_i, Cx_j\rangle$ as
\[
\langle Cx_i, Cx_j\rangle = \langle CP_{x_j}(x_i), Cx_j\rangle + \langle C\left(x_i - P_{x_j}(x_i)\right), Cx_j \rangle
\]
With a probability $1 - \exp(-\epsilon m/4)$, we have
\[
\left|\langle CP_{x_j}(x_i), Cx_j\rangle\right| \leq (1+\epsilon)\delta\beta
\]
With a probability $1 - 2\exp(-2\sqrt{m})$
\[
\left|\langle C\left(x_i - P_{x_j}(x_i)\right), Cx_j \rangle\right| \leq \frac{\beta}{m^{1/4}}
\]
\end{proof}


\subsection{Proof for Theorem~\ref{thm:linear_rate_convergence} [WIP]}
\begin{proof} \label{proof:thm_linear_rate}
All is left now is to find the network width and depth for which assumption~(\ref{eqn:gamma-upper-bound}) holds,
that is $\beta^2 \gamma n  \leq \alpha^2/2$. Revisiting~(\ref{eqn:gamma_value}), we need condition,
\begin{eqnarray}
    \gamma = C''\left(\left(m^{1/4}L\tau \right)^2 + \delta\left(\frac{5}{6}\right)^L + \frac{1}{m^{1/2}}\right)=O\left(\frac{1}{n} \right)
\end{eqnarray}
To meet the above condition, we need 
\[
    m^{1/4}L\tau = O\left(\frac{1}{\sqrt{n}}\right), \quad L=\Omega(\log n), \quad m = \Omega(n^2).
\]
Lemma~\ref{lemma:tao_bound} provides a bound for $\tau$, therefore,
% \begin{eqnarray*} \label{eqn:tau_val}
% \tau = \max\limits_{1 \leq t \leq T}\max\limits_{k\in [L]} \nm{W_{t,k}-W_{1,k}}_2 &\leq& \sum_{t=1}^{T-1}\max\limits_{k\in [L]} \nm{W_{t+1,k}-W_{t,k}}_2 \\
% &=& \eta\sum_{t=1}^{T-1}\max\limits_{k\in [L]} \nm{\nabla_k\ell(W_t)}_2 \\
% &\leq& \sqrt{3}\eta\beta\sum_{t=1}^{T-1}\sqrt{\ell(W_t)} \\
% &\leq& \sqrt{3\ell(W_1)}\eta\beta\sum_{t=0}^{T-1}\left(1-\frac{\eta\alpha^2 L}{4}\right)^{\frac{t}{2}} \\
% &\leq& \frac{8\sqrt{3\ell(W_1)}\beta}{\alpha^2L }
% \end{eqnarray*}



% Given a number of iterations $T_{\varepsilon}$, the variation of weights is bounded $\eta T_{\varepsilon}\geq \tau_{\varepsilon}$.
% To obtain accuracy $\varepsilon$, the number of iterations we need based on (\ref{eqn:linear_rate}) is,
% \begin{eqnarray} \label{eqn:tau_bound}
%     T_{\varepsilon} \leq \frac{4}{\eta\alpha^2 L}\log\frac{1}{\varepsilon} \quad \Longrightarrow \quad \tau_{\varepsilon}  \leq \frac{4}{\alpha^2 L}\log\frac{1}{\varepsilon} \label{eqn:tau_val}
% \end{eqnarray}
%\asaf{Q: why $\tau=\eta T$? A: T/eta is smaller than the max variation.}    
%\asaf{why $\alpha^2$ leads to $4/3$?}
%     \Omega\left(\frac{d}{mL}\log\frac{1}{\varepsilon}\right)
% \]
%and therefore $m^{1/4}L\tau \leq O(d/m^{3/4})$, implying
%  Therefore in order to meet the condition
\[
O\left(\frac{m^{\frac{1}{4}}\sqrt{\ell(W_1)}\beta L}{\alpha^2L} \right)
=O\left(d m^{-\frac{3}{4}}\sqrt{\ell(W_1)} \right)=O\left(\frac{1}{\sqrt{n}}\right), \quad m=\Omega \left((\ell(W_1)n)^{\frac{2}{3}}d^{\frac{4}{3}}\right)
\]
% \[
% O\left(\frac{m^{\frac{1}{4}}\log\frac{1}{\varepsilon}}{\alpha^2} \right)
% =O\left(\frac{m^{\frac{1}{4}}d^2}{m^2} \right)=O\left(\frac{1}{\sqrt{n}}\right), \quad m=\Omega \left((n^{\frac{1}{4}}d)^{\frac{8}{7}}\right)
% \]
% Therefore as long as $d\ll n^{\frac{3}{2}}$, the active condition for the width is $m = \Omega(n^2)$ (otherwise $m = \Omega\left(\max{\braces{n^2,(n^{\frac{1}{4}}d)^{\frac{8}{7}}}}\right)$).
Revisiting~(\ref{eqn:eta_min}), since $\frac{\alpha}{\beta}$ is constant and $\alpha>1$, and under assumption~(\ref{assum:labels}) $\ell(W_1)=O\left(nd\right)$, we can conclude that 
\[
\eta = \Theta\left((\beta^4L)^{-1}\right), \quad T_{\varepsilon}=O\left(\frac{m^2}{d^2} \log\frac{1}{\varepsilon} \right)=O\left(\frac{n^4}{d^2} \log\frac{1}{\varepsilon} \right)
\]



Where we used $\log(1-x)>-x$ to derive $T_{\varepsilon}$ from equation (\ref{eqn:linear_rate}).
\end{proof}



% \begin{lemma} \label{lemma:z-ka-kb-t}
% Under the following assumption,
% \[
%     \sqrt{3}e^{\epsilon/2}m^{1/4}L\tau \leq \frac{1}{9}
% \]
% %Then, for any
% with some $\epsilon \in (0, 1/5)$. Then, for any $1 \leq k_b < k_b \leq L$, with a probability larger than $1 - L^2\sqrt{m}\exp\left(-\epsilon m/[4L] + 6\sqrt{m}\right)$ we have
% \[
%     \|Z_{k_a, k_b}^t\|_2 \leq 5e^{\epsilon/2}m^{1/4}
% \]
% \end{lemma}
% \begin{proof}
% Define $Z_{k,k'} = D_k^iW_{1,k}\ldots W_{1,k'+1}D_{k'}^i$
% and $\delta W_{t,k} = W_{t,k} - W_{1,t}$. Expand $Z^t_{k_a, k_b}$ as
% \begin{eqnarray*}
% Z_{k_a,k_b}^t = Z_{k_a, k_b} + \sum_{s=1}^{k_b - k_a} \sum_{k_1 > k_2 >\ldots > k_s}Z_{k_a, k_1+1}\prod_{\ell=1}^s\delta W_{t,k_{\ell}}Z_{k_{\ell}+1, k_{\ell+1}}
% \end{eqnarray*}
% According to Lemma~\ref{lemma:z-ka-kb}, for any $\epsilon \in (0, 1/5)$, with a probability $1 - \sqrt{m}\exp\left(-\epsilon m/[4L] + 6\sqrt{m}\right)$, we have $\|Z_{k,k'}\| \leq \sqrt{3}m^{1/4}e^{\epsilon/2}$. We thus have, with a probability $1 - L^2\sqrt{m}\exp\left(-\epsilon m/[4L] + 6\sqrt{m}\right)$, \begin{eqnarray*}
% \|Z^t_{k_a, k_b}\|_2 \leq \sqrt{3}e^{\epsilon/2}m^{1/4}\left(1 + \sum_{s=1}^L \left[\sqrt{3}e^{\epsilon/2}m^{1/4}L\tau\right]^s\right) \leq \sqrt{3}e^{\epsilon/2}m^{1/4}\left(1 + \frac{1}{1 - \sqrt{3}e^{\epsilon/2}m^{1/4}L\tau}\right)
% \end{eqnarray*}
% Since
% \[
% \sqrt{3}e^{\epsilon/2}m^{1/4}L\tau \leq \frac{1}{9}
% \]
% \asaf{I think the it should be $c(1+\frac{q}{1-q})$ so $\frac{9\sqrt{3}}{8}$ and not $\frac{17\sqrt{3}}{8}$, and below $5\rightarrow 2$}
% we have
% \[
%     \|Z^t_{k_a, k_b}\|_2 \leq 5e^{\epsilon/2}m^{1/4}
% \]
% \end{proof}

%----------------------------------------------------
% {\bf\color{red} The below is a new result for the bound of $|Z_{k_a, k_b}|_2$. I just realized that the entire proof can remain unchanged except that I need to divide each vector of $m$ dimension into $\log^2m$ chunks. The reason I have to divide each vector into $\log^2m$ chunks is $L = \log n$ and $m = \Omega(n)$. Hence, only when dividing each vector into $\log^2m$ chunks, we can guarantee $\epsilon m/[4L] - 6m/\log^2m \geq \Omega(m/L)$ holds.}
%-----------------------------------------------
